# Supplementary material for: No Reason for No Supervision: Improved Generalization in Supervised Models
Source: arXiv:2206.15369 source file (2023-03-10)
Supplement: Supplementary file 1 [file related_work_extended.tex]

\section{Extended related work}\label{sec:relwork_extended}

\mbs{
This is the related work section we had in arxiv plus an extended discussion on~\cite{wang2022revisiting} at the end.
Revisit this section after the related work section of the main paper is finalized.
This section shouldn't overlap with the one in the main paper.
}

\looseness=-1
Soon after the remarkable performance of AlexNet~\citep{krizhevsky2012alexnet} on \imnet{}, the computer vision community started leveraging the fact that representations produced by deep networks trained for \imnet classification transfer to other datasets and tasks~\citep{donahue2014decaf,razavian2014cnn}.
Several works since then have proposed practical transfer approaches~\citep{goyal2019scaling,pandy2022transferability,zhai2019large}, while others have contributed to a formal understanding of those beneficial generalization properties~\citep{huh2016what,kornblith2019transfer,tripuraneni2020theory,yosinski2014how}.
Recent work in this context~\citep{kornblith2021why,sariyildiz2021cog} has shown that the best representations for \imnet were not necessarily the ones transferring best.
For instance, some regularization techniques or loss functions improving \imnet classification lead to underwhelming transfer results~\citep{kornblith2021why,sariyildiz2021cog}.
A parallel line of work based on self-supervised learning~\citep{caron2020swav,chen2020simclr,grill2020byol,he2020moco} focused on training models without manual labels, and demonstrated their strong generalization capabilities to many transfer datasets, clearly surpassing their supervised counterparts~\citep{sariyildiz2021cog}.
Yet, as expected, SSL models are no match to the supervised models on the \imnet{} classification task itself.

A few approaches have tackled the task of training supervised models that also transfer well and share motivation with our work.
SupCon~\citep{khosla2020supcon} extends SimCLR~\citep{chen2020simclr} using image labels to build positive pairs.
As such, its formulation is close to neighborhood component analysis (NCA)~\citep{goldberger2004neighbourhood}.
It circumvents the need for large batches by adding a momentum and a memory similar to MoCo~\citep{he2020moco}.
Supervised-MoCo~\citep{zhao2021whatmakes} filters out false negatives in the memory bank of MoCo using image labels, while LOOK~\citep{feng2022rethinking} modifies the NCA objective to only consider the closest neighbors of each query image.
We experimentally observe that our model design leads to better transfer than all these works.

Our work is also related to the metric learning literature.
Metric learning models are trained with labels but evaluated on unseen concepts, and often focus on specific and narrow class domains such as bird species or car models~\citep{qian2019softtriple,sohn2016improved,zheng2021deep}.
Therefore, they are not directly applicable to our problem.
Moreover, their formulation usually involves computing pairwise image similarities~\citep{movshovitz2017nofuss,wu2018improving}, which does not scale to \imnet.
Also related, adversarially robust classifiers have been shown to transfer well~\citep{salman2020adversarially}, but the level of noise applied during training needs to be carefully set for each task.

\looseness=-1
Departing from all these methods, we propose an effective training setup, which leverages multi-crop augmentation~\citep{caron2020swav} and an expendable projector head~\citep{chen2020simclr}, two key components in many successful SSL approaches~\citep{caron2021dino,chen2020mocov2,chen2021simsiam,grill2020byol}.
Multi-crop is typically used for creating diverse and challenging views of an image, for which the model is encouraged to learn consistent representations~\citep{assran2021semi,caron2021dino}.
A concurrent work~\citep{wang2022importance} argues that multi-crop increases representation variance and should be used for online self-distillation, while it has recently been shown to also improve vision and language pretraining~\citep{ko2022large}.
We show that this design works out-of-the-box also for supervised training on \imnet.

\looseness=-1
The use of expendable projectors comes from the observation that the last layer of a model is not necessarily the one producing features that transfer best.
Early works on SSL evaluate representations from multiple layers throughout the model~\citep{goyal2019scaling,kolesnikov2019revisiting,zhang2016colorful}, as the last layer tends to overfit to the proxy task, \eg clustering~\citep{caron2018deep} or rotation prediction~\citep{gidaris2018rotnet}.
To train more generic features, SimCLR~\citep{chen2020simclr} adds a MLP projector after the encoder, that is discarded later.
This design has become standard practice in SSL~\citep{caron2021dino,chen2020mocov2,grill2020byol,zbontar2021barlow}.
Projectors are also used in recent supervised models such as SupCon~\citep{khosla2020supcon} and LOOK~\citep{feng2022rethinking}, but none of these works studies the impact of the projector design choices on representation quality.
\mbst{
A notable exception is the recent work of~\citet{wang2022revisiting}, which shows that training supervised models using a projector improves their transfer learning performance.
Different from this work, we extend the scope of projectors by also considering the performance on the original \imnet task.
We show (in~\Cref{sec:exp}) that depending on the size of the projector, there exists a trade-off between \imnet and transfer performance, which is not obvious to see in \citet{wang2022revisiting} as it mainly focuses on transfer performance and explores projectors with 1 hidden layer.
Also, we show that gains from projectors are complementary to multi-crop as well as alternative training objectives.
Our models reach state-of-the-art in transfer learning outperforming the recent self- and semi-supervised DINO and PAWS models.
}
