# Supplementary material for: No Reason for No Supervision: Improved Generalization in Supervised Models
Source: arXiv:2206.15369 source file (2023-03-10)
Supplement: Supplementary file 2 [file fig_singular_values.tex]

\begin{figure}
    \centering
    \begin{subfigure}{\linewidth}
        \includegraphics[width=\linewidth]{res/singular_values_1000_per_dataset.pdf}
        \caption{
            For the {\bf top 1000 dimensions}.
        }
        \label{fig:singular_values_1000_per_dataset}
    \end{subfigure}
    \begin{subfigure}{\linewidth}
        \includegraphics[width=\linewidth]{res/singular_values_0100_per_dataset.pdf}
        \caption{
            For the {\bf top 100 dimensions}.
        }
        \label{fig:singular_values_100_per_dataset}
    \end{subfigure}
    \caption{
        \mbst{
        {\bf Singular values} sorted w.r.t. their magnitude for the pre-extracted features of the 4 models from~\Cref{fig:pwise_dist_sparsity}.
        }
    }
    \label{fig:singular_values_per_dataset}
\end{figure}
